# Supplementary material for: Delayed Reinforcement Learning by Imitation
Source: arXiv:2205.05569 source file (2022-05-11)
Supplement: Supplementary file 1 [file 4_imitation_bound.tex]

\begin{thm}
\label{th:state_distrib_imitation}
    Consider an $(L_P,L_r)$-LC MDP $\mathcal{M}$ and two policies $\pi_E$ and $\pi_I$ with $\pi_E$ Lipschitz with parameter $L_\pi$.
    Then, 
    $$\mathcal W_1(d_{s}^{\pi_E},d_{s}^{\pi_I})\le \frac{1}{1-\gamma L_p (1+L_\pi)}\mathcal W_1(\pi_E(\cdot|s),\pi_I(\cdot|s))$$
\end{thm}
\begin{proof}
By \cite{mdp:kakade02}, for every policy $\pi$,
$$d_s^\pi(z) = (1-\gamma)\delta_s(z) +
    \gamma \int_A \int_S d^\pi_s(s')\pi(a'|s')p(z|s',a')ds'\ da'.$$
Applying this theorem to both policies, we have
\begin{align*}\mathcal W_1(d_{s}^{\pi_E},d_{s}^{\pi_I})=&
            \sup_{\|f\|_L=1}  \int_S f(z) \bigg ( (1-\gamma)\delta_s(z) +
    \gamma \int_A \int_S d^{\pi_E}_s(s')\pi_E(a'|s')p(z|s',a')ds'\ da'\\
    &-(1-\gamma)\delta_s(z) -
    \gamma \int_A \int_S d^{\pi_I}_s(s')\pi_I(a'|s')p(z|s',a')ds'\ da'\bigg ) dz =\\
    &=\sup_{\|f\|_L=1} \int_S f(z) \bigg (
    \gamma \int_A \int_S \Big (d^{\pi_E}_s(s')\pi_E(a'|s')-d^{\pi_I}_s(s')\pi_I(a'|s')\Big )p(z|s',a')ds'\ da'\bigg ) dz
\end{align*}

Now, exchanging the order of integration, we have

$$\sup_{\|f\|_L=1}  
    \gamma \int_A \int_S \Big (d^{\pi_E}_s(s')\pi_E(a'|s')-d^{\pi_I}_s(s')\pi_I(a'|s')\Big )\Big (\int_S f(z)p(z|s',a')dz \Big ) ds'\ da' $$
    
We then add and subtract $d^{\pi_E}_s(s')\pi_I(a'|s')$, getting that the former is the sum of two terms. First,

$$\sup_{\|f\|_L=1}  
    \gamma \int_A \int_S d^{\pi_E}_s(s')\Big (\pi_E(a'|s')-\pi_I(a'|s')\Big )\Big (\int_S f(z)p(z|s',a')dz \Big ) ds'\ da' $$
    
which, being $\int_S f(z)p(z|s',a')dz$ $L_P$ Lipschitz w.r.t. $a'$, is bounded by $\gamma L_P\E_{s'\sim d^{\pi_E}_s(\cdot)}[\mathcal W_1(\pi_E(\cdot|s'),\pi_I(\cdot|s'))]$.

Second, we have 

$$\sup_{\|f\|_L=1}  
    \gamma \int_S \Big (d^{\pi_E}_s(s')-d^{\pi_I}_s(s')\Big )\int_S\int_A \pi_I(a'|s') f(z)p(z|s',a')dz  \ da'\ ds' $$

Then, by \ref{pp:lip_g}), the function $\int_S\int_A \pi_I(a'|s') f(z)p(z|s',a')dz\ da'$ is $L_P(1+L_\pi)$ Lipschitz. So, the former is bounded by

$$\sup_{\|g\|_L=L_P(1+L_\pi)}  
    \gamma \int_S \Big (d^{\pi_E}_s(s')-d^{\pi_I}_s(s')\Big )g(s')\ ds'=\gamma L_P(1+L_\pi)\mathcal W_1(d_{s}^{\pi_E},d_{s}^{\pi_I})$$
    
Putting together both sides, we have

$$\mathcal W_1(d_{s}^{\pi_E},d_{s}^{\pi_I}) \le \gamma L_P\E_{s'\sim d^{\pi_E}_s(\cdot)}[\mathcal W_1(\pi_E(\cdot|s'),\pi_I(\cdot|s'))] + \gamma L_P(1+L_\pi)\mathcal W_1(d_{s}^{\pi_E},d_{s}^{\pi_I})$$

which entails

$$\mathcal W_1(d_{s}^{\pi_E},d_{s}^{\pi_I}) \le \frac{\gamma L_P}{1-\gamma L_P(1+L_\pi)}\E_{s'\sim d^{\pi_E}_s(\cdot)}[\mathcal W_1(\pi_E(\cdot|s'),\pi_I(\cdot|s'))]$$

\end{proof}

\begin{thm}\label{th:imitation_bound}
    Consider an $(L_P,L_r)$-LC MDP $\mathcal{M}$ and two policies $\pi_E$ and $\pi_I$ with $\pi_E$ Lipschitz with parameter $L_\pi$.
    Then,
    $$V^{\pi_E}(s)-V^{\pi_I}(s)$$
\end{thm}
\begin{proof}
    $$V^{\pi_E}(s)-V^{\pi_I}(s)=\frac{1}{1-\gamma}\int_S \int_A r(s',a)\pi_E(a|s')d_{s}^{\pi_E}(s')\ ds'-\int_S \int_A r(s',a)\pi_I(a|s')d_{s}^{\pi_I}(s')\ ds'$$
    
    where we can do the following passages:
    \begin{align*}
        V^{\pi_E}(s)-V^{\pi_I}(s)=&\frac{1}{1-\gamma}\int_S \int_A r(s',a)\Big (\pi_E(a|s')d_{s}^{\pi_E}(s')-\pi_I(a|s')d_{s}^{\pi_I}(s')\Big )\ ds'\\
        =& \frac{1}{1-\gamma}\int_S \int_A r(s',a)\pi_I(a|s')\Big (d_{s}^{\pi_E}(s')-d_{s}^{\pi_I}(s')\Big )\ ds'+\\
        & \frac{1}{1-\gamma}\int_S \int_A r(s',a)d_{s}^{\pi_E}(s')\Big (\pi_E(a|s')-\pi_I(a|s')\Big )\ ds'\\
        \le &\frac{1}{1-\gamma} L_rL_{\pi_I}\mathcal W_1(d_{s}^{\pi_E},d_{s}^{\pi_I}) + \frac{1}{1-\gamma}L_r
        \E_{s'\sim d^{\pi_E}_s(\cdot)}[\mathcal W_1(\pi_E(\cdot|s'),\pi_I(\cdot|s'))]\\
        =&\frac{L_r}{1-\gamma}\frac{\gamma L_P+L_{\pi_I}(1-\gamma L_P(1+L_\pi))}{1-\gamma L_P(1+L_\pi)}\E_{s'\sim d^{\pi_E}_s(\cdot)}[\mathcal W_1(\pi_E(\cdot|s'),\pi_I(\cdot|s'))]
    \end{align*}
\end{proof}
